# Supplementary material for: Markov Decision Process modeled with Bandits for Sequential Decision Making in Linear-flow
Source: arXiv:2107.00204 source file (2022-03-16)
Supplement: Supplementary file 1 [file appendix.tex]

Too add later.
